# Supplementary material for: DyST-XL: Dynamic Layout Planning and Content Control for Compositional Text-to-Video Generation
Source: arXiv:2504.15032 source file (2025-04-30)
Supplement: Supplementary file 1 [file supp.tex]

\section{Supplementary Materials}

\subsection{More Results}
\textbf{The prompt of LLM Planner.} We provide the instruction prompt of LLM Planner, as shown in \cref{fig:LLM-planner}.

\begin{figure*}[!h]
    \centering
    \includegraphics[width=0.75\linewidth]{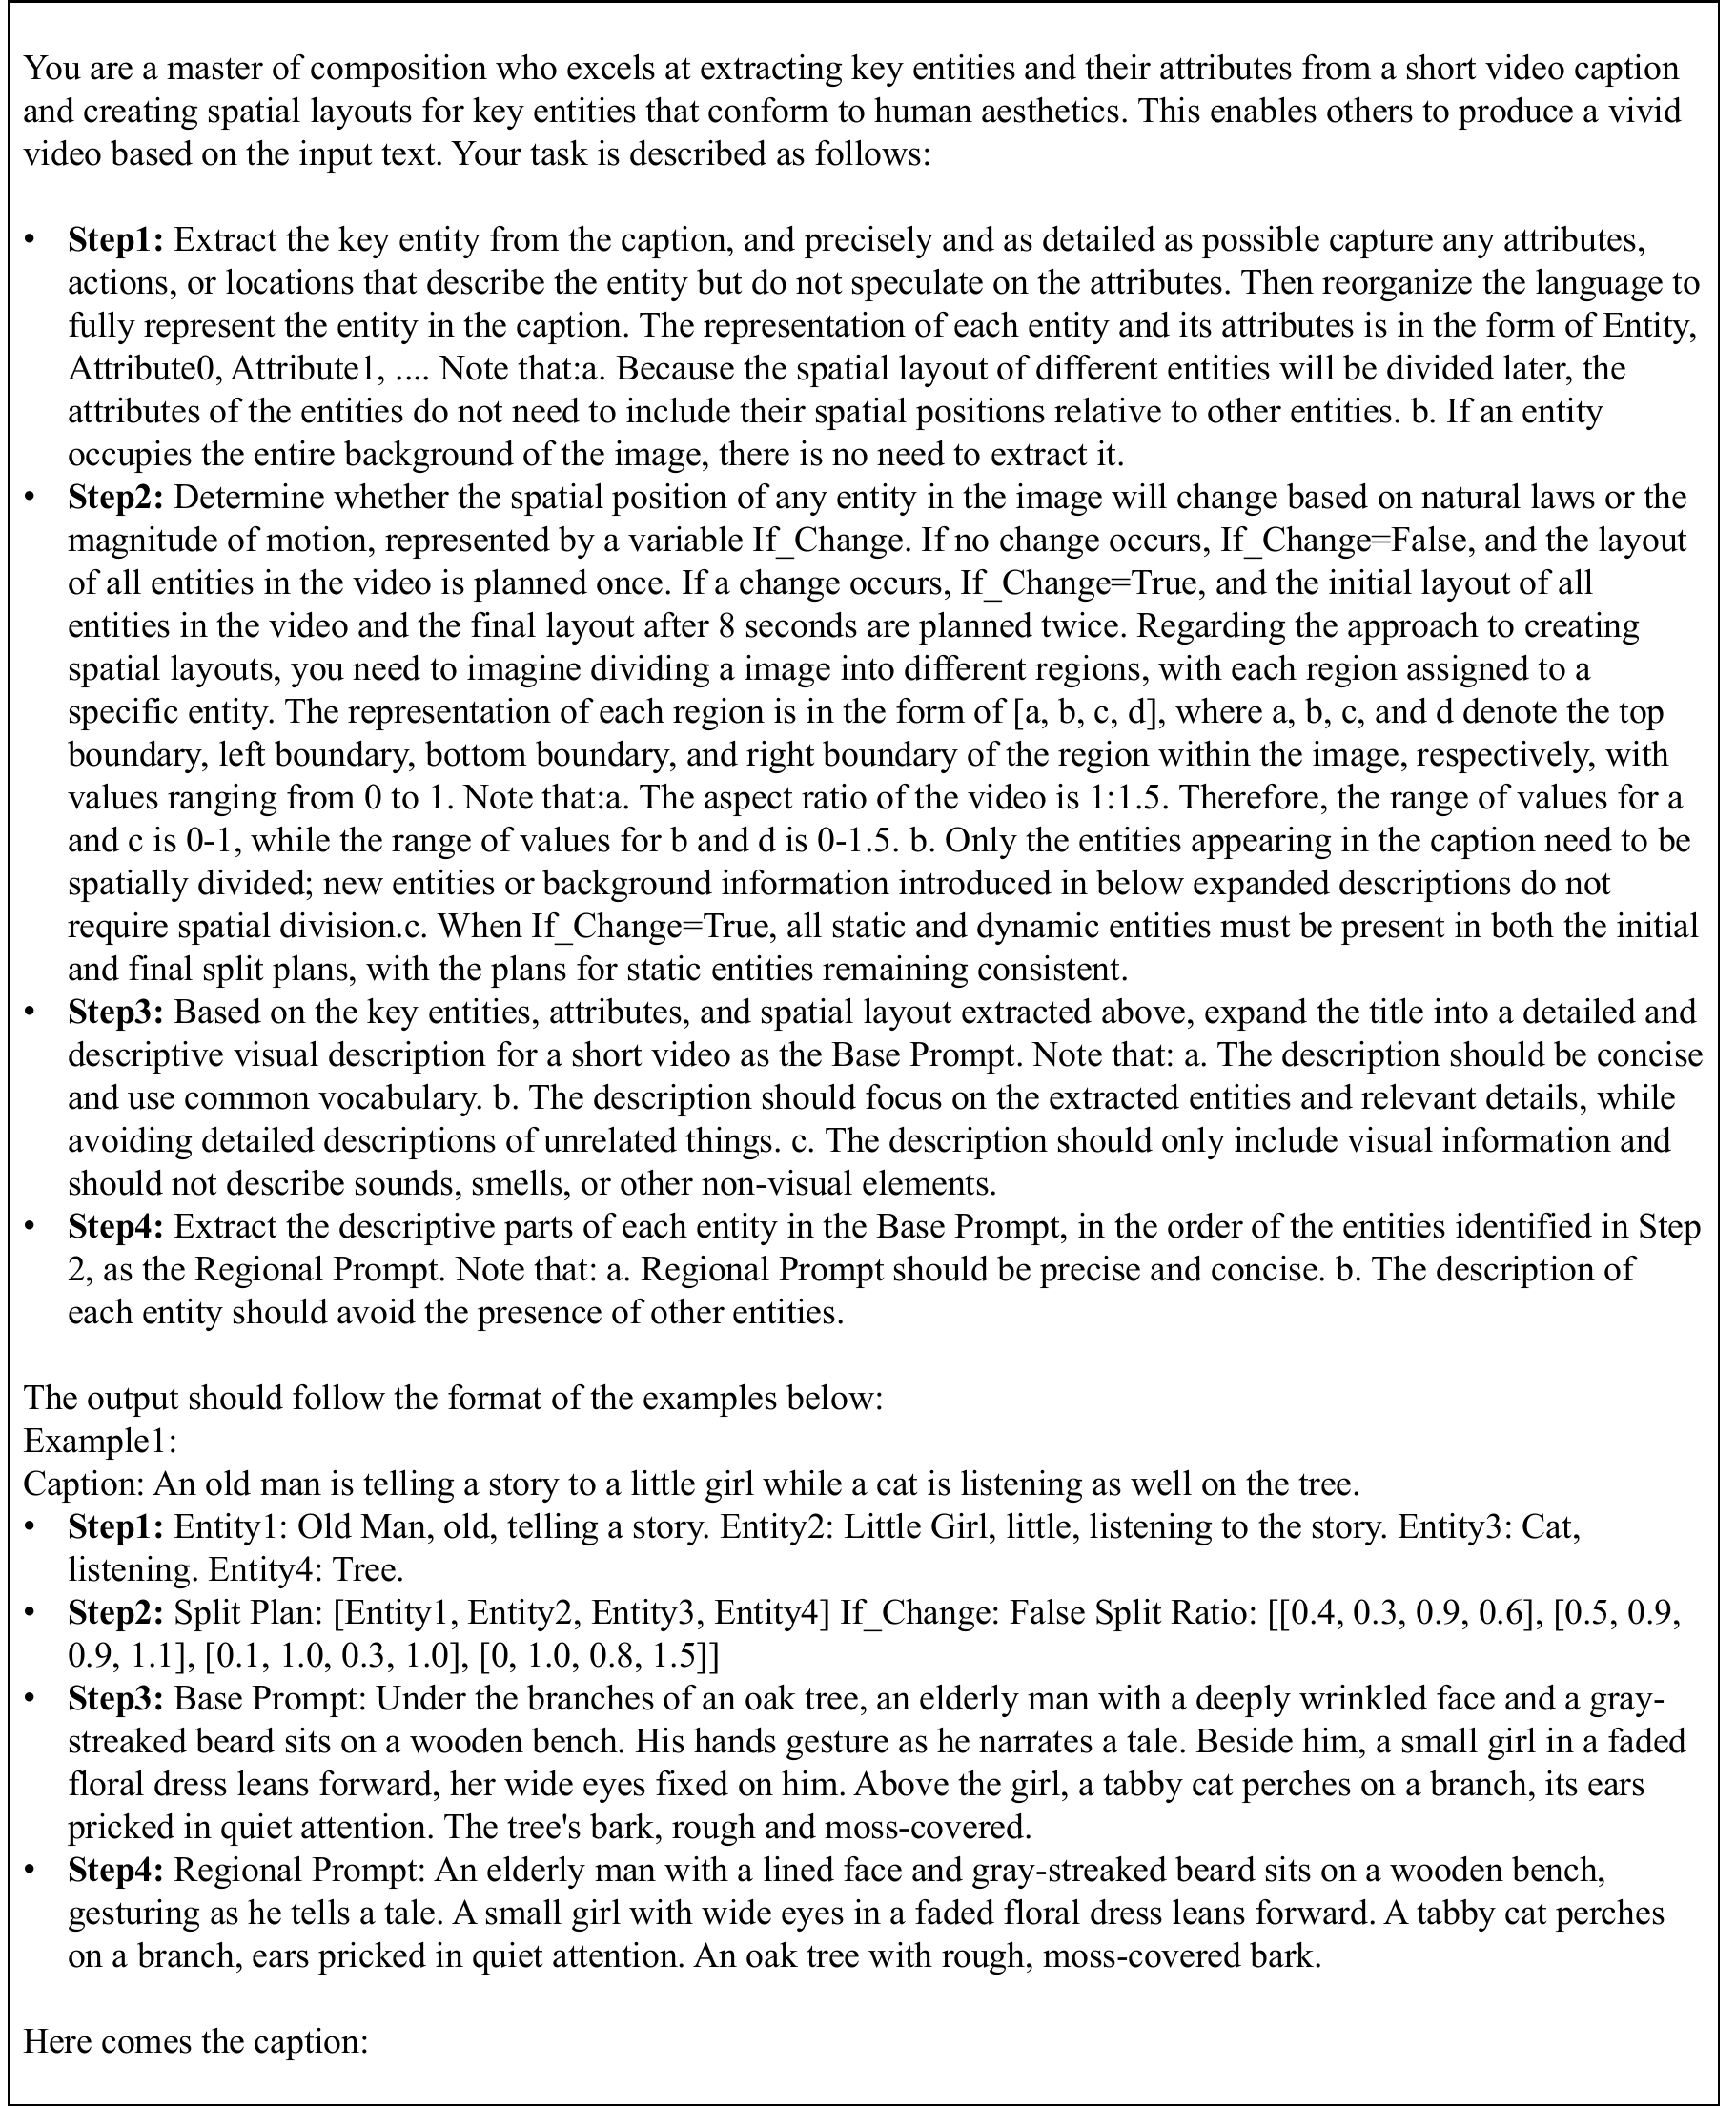}
    \caption{Instruction prompt for LLM Planner.}
    \label{fig:LLM-planner}
\end{figure*}

\textbf{Videos.} We provide the detail videos on \textbf{\textit{the folder of videos}}.
